# Supplementary material for: Consistency and Accuracy of CelebA Attribute Values
Source: arXiv:2210.07356 source file (2023-04-16)
Supplement: Supplementary file 1 [file information_not_visible.tex]

\begin{figure}[h]
    \centering
    \begin{subfigure}[b]{1\linewidth}
    \captionsetup[subfigure]{labelformat=empty}
        \begin{subfigure}[b]{1\linewidth}
            \begin{subfigure}[b]{1\linewidth}
            \centering
                \begin{subfigure}[b]{0.15\linewidth}
                    \includegraphics[width=\linewidth]{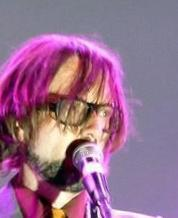}
                    
                \end{subfigure}
                \begin{subfigure}[b]{0.15\linewidth}
                    \includegraphics[width=\linewidth]{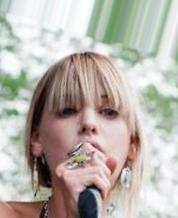}
                    
                \end{subfigure}
                \begin{subfigure}[b]{0.15\linewidth}
                    \includegraphics[width=\linewidth]{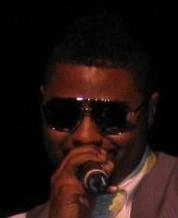}
                    
                \end{subfigure}
                \begin{subfigure}[b]{0.15\linewidth}
                    \includegraphics[width=\linewidth]{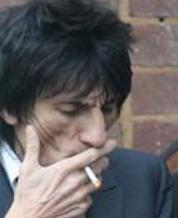}
                    
                \end{subfigure}
                \begin{subfigure}[b]{0.15\linewidth}
                    \includegraphics[width=\linewidth]{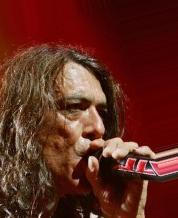}
                    
                \end{subfigure}
                \begin{subfigure}[b]{0.15\linewidth}
                    \includegraphics[width=\linewidth]{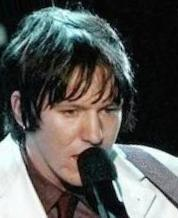}
                    
                \end{subfigure}
            \end{subfigure}
            \begin{subfigure}[b]{1\linewidth}
            \centering
                \begin{subfigure}[b]{0.15\linewidth}
                    \includegraphics[width=\linewidth]{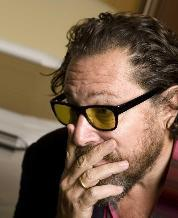}
                    
                \end{subfigure}
                \begin{subfigure}[b]{0.15\linewidth}
                    \includegraphics[width=\linewidth]{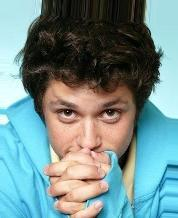}
                    
                \end{subfigure}
                \begin{subfigure}[b]{0.15\linewidth}
                    \includegraphics[width=\linewidth]{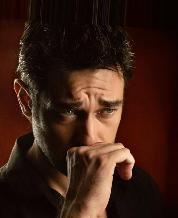}
                    
                \end{subfigure}
                \begin{subfigure}[b]{0.15\linewidth}
                    \includegraphics[width=\linewidth]{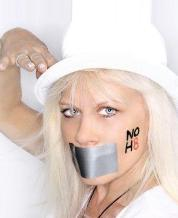}
                    
                \end{subfigure}
                \begin{subfigure}[b]{0.15\linewidth}
                    \includegraphics[width=\linewidth]{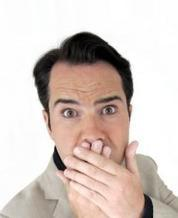}
                    
                \end{subfigure}
                \begin{subfigure}[b]{0.15\linewidth}
                    \includegraphics[width=\linewidth]{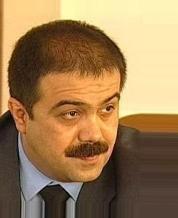}
                    
                \end{subfigure}
            \end{subfigure}
        \end{subfigure}
        
        \begin{subfigure}[b]{1\linewidth}
            \begin{subfigure}[b]{1\linewidth}
            \centering
                \begin{subfigure}[b]{0.15\linewidth}
                    \includegraphics[width=\linewidth]{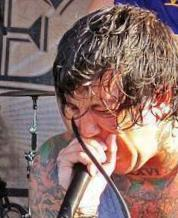}
                    
                \end{subfigure}
                \begin{subfigure}[b]{0.15\linewidth}
                    \includegraphics[width=\linewidth]{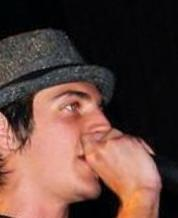}
                    
                \end{subfigure}
                \begin{subfigure}[b]{0.15\linewidth}
                    \includegraphics[width=\linewidth]{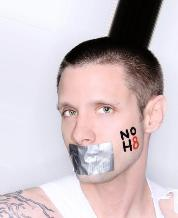}
                    
                \end{subfigure}
                \begin{subfigure}[b]{0.15\linewidth}
                    \includegraphics[width=\linewidth]{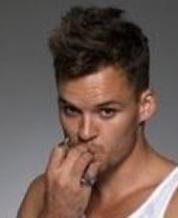}
                    
                \end{subfigure}
                \begin{subfigure}[b]{0.15\linewidth}
                    \includegraphics[width=\linewidth]{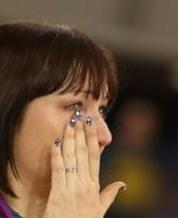}
                    
                \end{subfigure}
                \begin{subfigure}[b]{0.15\linewidth}
                    \includegraphics[width=\linewidth]{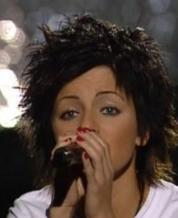}
                    
                \end{subfigure}
            \end{subfigure}
            \begin{subfigure}[b]{1\linewidth}
            \centering
                \begin{subfigure}[b]{0.15\linewidth}
                    \includegraphics[width=\linewidth]{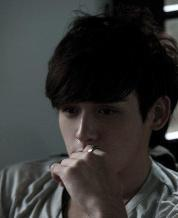}
                    
                \end{subfigure}
                \begin{subfigure}[b]{0.15\linewidth}
                    \includegraphics[width=\linewidth]{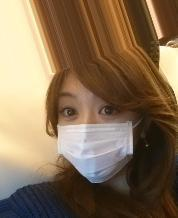}
                    
                \end{subfigure}
                \begin{subfigure}[b]{0.15\linewidth}
                    \includegraphics[width=\linewidth]{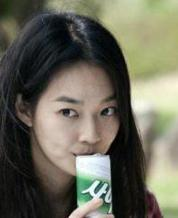}
                    
                \end{subfigure}
                \begin{subfigure}[b]{0.15\linewidth}
                    \includegraphics[width=\linewidth]{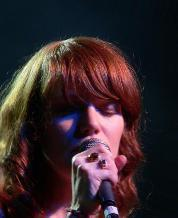}
                    
                \end{subfigure}
                \begin{subfigure}[b]{0.15\linewidth}
                    \includegraphics[width=\linewidth]{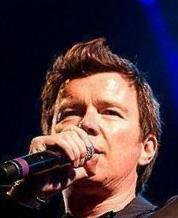}
                    
                \end{subfigure}
                \begin{subfigure}[b]{0.15\linewidth}
                    \includegraphics[width=\linewidth]{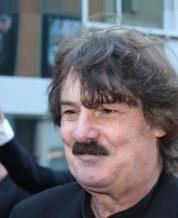}
                    
                \end{subfigure}
            \end{subfigure}
        \end{subfigure}
        
        \begin{subfigure}[b]{1\linewidth}
            \begin{subfigure}[b]{1\linewidth}
            \centering
                \begin{subfigure}[b]{0.15\linewidth}
                    \includegraphics[width=\linewidth]{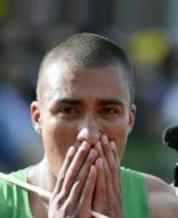}
                    
                \end{subfigure}
                \begin{subfigure}[b]{0.15\linewidth}
                    \includegraphics[width=\linewidth]{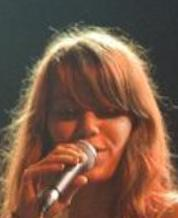}
                    
                \end{subfigure}
                \begin{subfigure}[b]{0.15\linewidth}
                    \includegraphics[width=\linewidth]{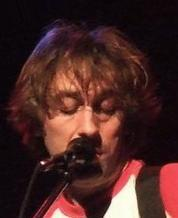}
                    
                \end{subfigure}
                \begin{subfigure}[b]{0.15\linewidth}
                    \includegraphics[width=\linewidth]{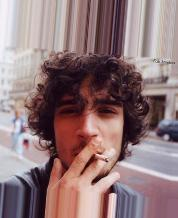}
                    
                \end{subfigure}
                \begin{subfigure}[b]{0.15\linewidth}
                    \includegraphics[width=\linewidth]{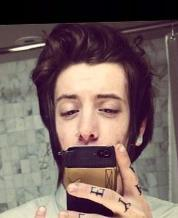}
                    
                \end{subfigure}
                \begin{subfigure}[b]{0.15\linewidth}
                    \includegraphics[width=\linewidth]{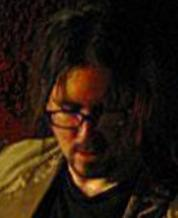}
                    
                \end{subfigure}
            \end{subfigure}
            \begin{subfigure}[b]{1\linewidth}
            \centering
                \begin{subfigure}[b]{0.15\linewidth}
                    \includegraphics[width=\linewidth]{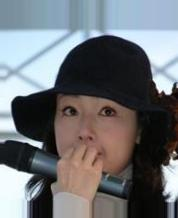}
                    
                \end{subfigure}
                \begin{subfigure}[b]{0.15\linewidth}
                    \includegraphics[width=\linewidth]{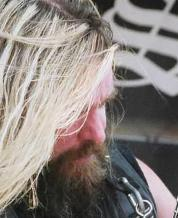}
                    
                \end{subfigure}
                \begin{subfigure}[b]{0.15\linewidth}
                    \includegraphics[width=\linewidth]{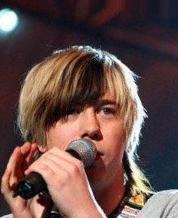}
                    
                \end{subfigure}
                \begin{subfigure}[b]{0.15\linewidth}
                    \includegraphics[width=\linewidth]{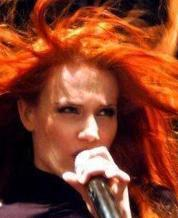}
                    
                \end{subfigure}
                \begin{subfigure}[b]{0.15\linewidth}
                    \includegraphics[width=\linewidth]{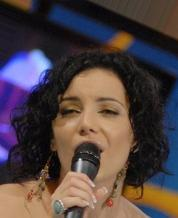}
                    
                \end{subfigure}
                \begin{subfigure}[b]{0.15\linewidth}
                    \includegraphics[width=\linewidth]{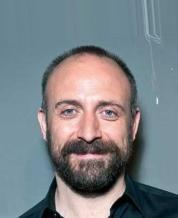}
                    
                \end{subfigure}
            \end{subfigure}
            
            \begin{subfigure}[b]{1\linewidth}
            \centering
                \begin{subfigure}[b]{0.15\linewidth}
                    \includegraphics[width=\linewidth]{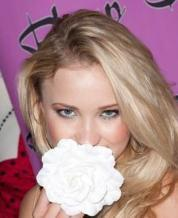}
                    
                \end{subfigure}
                \begin{subfigure}[b]{0.15\linewidth}
                    \includegraphics[width=\linewidth]{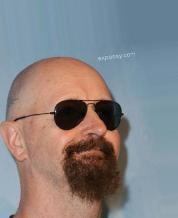}
                    
                \end{subfigure}
                \begin{subfigure}[b]{0.15\linewidth}
                    \includegraphics[width=\linewidth]{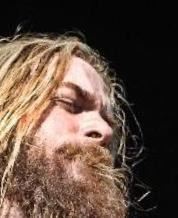}
                    
                \end{subfigure}
                \begin{subfigure}[b]{0.15\linewidth}
                    \includegraphics[width=\linewidth]{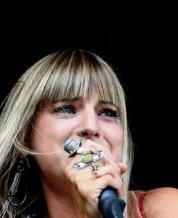}
                    
                \end{subfigure}
                \begin{subfigure}[b]{0.15\linewidth}
                    \includegraphics[width=\linewidth]{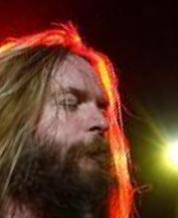}
                    
                \end{subfigure}
                \begin{subfigure}[b]{0.15\linewidth}
                    \includegraphics[width=\linewidth]{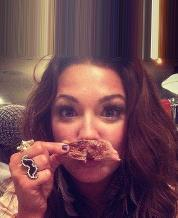}
                    
                \end{subfigure}
            \end{subfigure}
        \end{subfigure}
        
    \end{subfigure}
   \caption{Examples of the third annotation option: information not visible.}
\label{fig:imformation-not-visible}
\end{figure}
