# Supplementary material for: Consistency and Accuracy of CelebA Attribute Values
Source: arXiv:2210.07356 source file (2023-04-16)
Supplement: Supplementary file 4 [file inconsistent_definitions.tex]

\begin{figure}[h]
    \centering
    \begin{subfigure}[b]{1\linewidth}
    \captionsetup[subfigure]{labelformat=empty}
        \begin{subfigure}[b]{1\linewidth}
            \begin{subfigure}[b]{1\linewidth}
            \centering
                \begin{subfigure}[b]{0.15\linewidth}
                    \includegraphics[width=\linewidth]{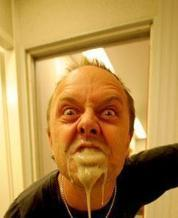}
                    
                \end{subfigure}
                \begin{subfigure}[b]{0.15\linewidth}
                    \includegraphics[width=\linewidth]{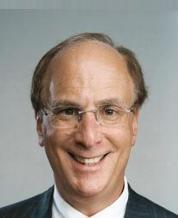}
                    
                \end{subfigure}
                \begin{subfigure}[b]{0.15\linewidth}
                    \includegraphics[width=\linewidth]{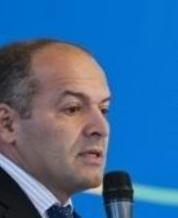}
                    
                \end{subfigure}
                \begin{subfigure}[b]{0.15\linewidth}
                    \includegraphics[width=\linewidth]{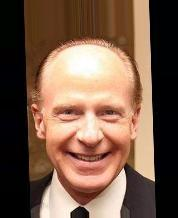}
                    
                \end{subfigure}
                \begin{subfigure}[b]{0.15\linewidth}
                    \includegraphics[width=\linewidth]{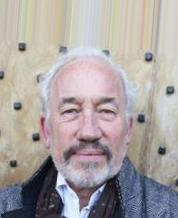}
                    
                \end{subfigure}
                \begin{subfigure}[b]{0.15\linewidth}
                    \includegraphics[width=\linewidth]{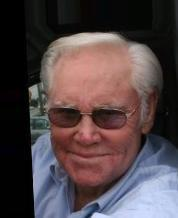}
                    
                \end{subfigure}
            \end{subfigure}
            \begin{subfigure}[b]{1\linewidth}
            \centering
                \begin{subfigure}[b]{0.15\linewidth}
                    \includegraphics[width=\linewidth]{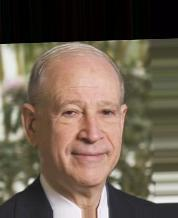}
                    
                \end{subfigure}
                \begin{subfigure}[b]{0.15\linewidth}
                    \includegraphics[width=\linewidth]{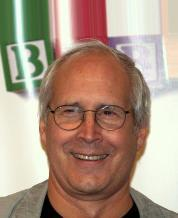}
                    
                \end{subfigure}
                \begin{subfigure}[b]{0.15\linewidth}
                    \includegraphics[width=\linewidth]{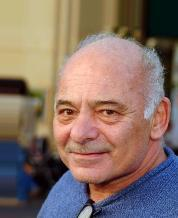}
                    
                \end{subfigure}
                \begin{subfigure}[b]{0.15\linewidth}
                    \includegraphics[width=\linewidth]{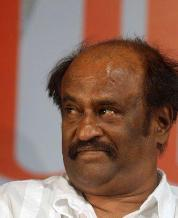}
                    
                \end{subfigure}
                \begin{subfigure}[b]{0.15\linewidth}
                    \includegraphics[width=\linewidth]{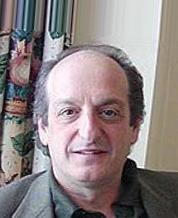}
                    
                \end{subfigure}
                \begin{subfigure}[b]{0.15\linewidth}
                    \includegraphics[width=\linewidth]{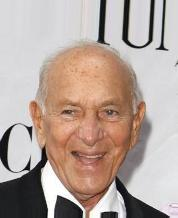}
                    
                \end{subfigure}
            \end{subfigure}
            \caption{Error samples of bald=true in original dataset}
        \end{subfigure}
        
        \begin{subfigure}[b]{1\linewidth}
            \begin{subfigure}[b]{1\linewidth}
            \centering
                \begin{subfigure}[b]{0.15\linewidth}
                    \includegraphics[width=\linewidth]{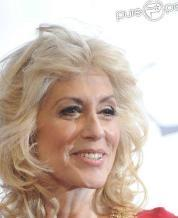}
                    
                \end{subfigure}
                \begin{subfigure}[b]{0.15\linewidth}
                    \includegraphics[width=\linewidth]{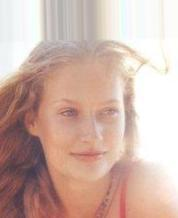}
                    
                \end{subfigure}
                \begin{subfigure}[b]{0.15\linewidth}
                    \includegraphics[width=\linewidth]{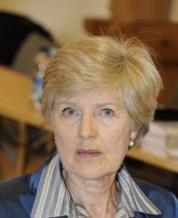}
                    
                \end{subfigure}
                \begin{subfigure}[b]{0.15\linewidth}
                    \includegraphics[width=\linewidth]{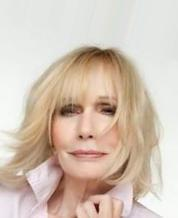}
                    
                \end{subfigure}
                \begin{subfigure}[b]{0.15\linewidth}
                    \includegraphics[width=\linewidth]{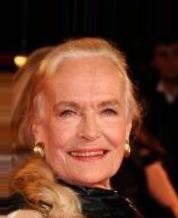}
                    
                \end{subfigure}
                \begin{subfigure}[b]{0.15\linewidth}
                    \includegraphics[width=\linewidth]{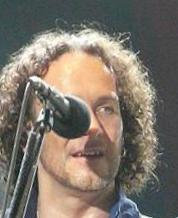}
                    
                \end{subfigure}
            \end{subfigure}
            \begin{subfigure}[b]{1\linewidth}
            \centering
                \begin{subfigure}[b]{0.15\linewidth}
                    \includegraphics[width=\linewidth]{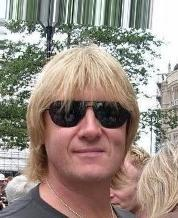}
                    
                \end{subfigure}
                \begin{subfigure}[b]{0.15\linewidth}
                    \includegraphics[width=\linewidth]{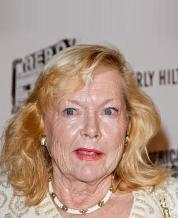}
                    
                \end{subfigure}
                \begin{subfigure}[b]{0.15\linewidth}
                    \includegraphics[width=\linewidth]{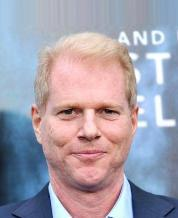}
                    
                \end{subfigure}
                \begin{subfigure}[b]{0.15\linewidth}
                    \includegraphics[width=\linewidth]{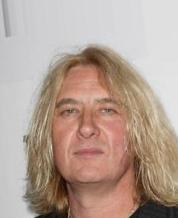}
                    
                \end{subfigure}
                \begin{subfigure}[b]{0.15\linewidth}
                    \includegraphics[width=\linewidth]{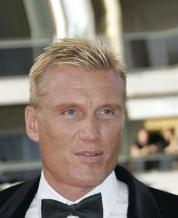}
                    
                \end{subfigure}
                \begin{subfigure}[b]{0.15\linewidth}
                    \includegraphics[width=\linewidth]{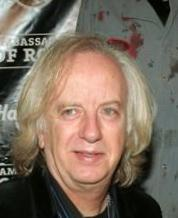}
                    
                \end{subfigure}
            \end{subfigure}
            \caption{Error samples of gray\_hair=true in original dataset}
        \end{subfigure}
        
        \begin{subfigure}[b]{1\linewidth}
            \begin{subfigure}[b]{1\linewidth}
            \centering
                \begin{subfigure}[b]{0.15\linewidth}
                    \includegraphics[width=\linewidth]{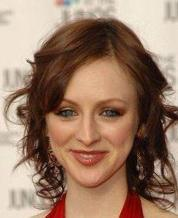}
                    
                \end{subfigure}
                \begin{subfigure}[b]{0.15\linewidth}
                    \includegraphics[width=\linewidth]{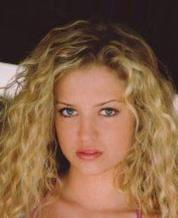}
                    
                \end{subfigure}
                \begin{subfigure}[b]{0.15\linewidth}
                    \includegraphics[width=\linewidth]{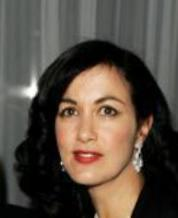}
                    
                \end{subfigure}
                \begin{subfigure}[b]{0.15\linewidth}
                    \includegraphics[width=\linewidth]{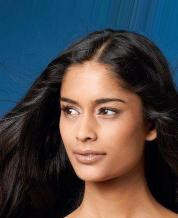}
                    
                \end{subfigure}
                \begin{subfigure}[b]{0.15\linewidth}
                    \includegraphics[width=\linewidth]{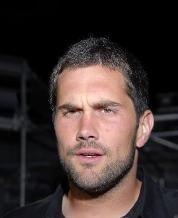}
                    
                \end{subfigure}
                \begin{subfigure}[b]{0.15\linewidth}
                    \includegraphics[width=\linewidth]{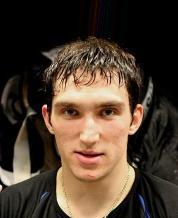}
                    
                \end{subfigure}
            \end{subfigure}
            \begin{subfigure}[b]{1\linewidth}
            \centering
                \begin{subfigure}[b]{0.15\linewidth}
                    \includegraphics[width=\linewidth]{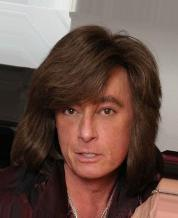}
                    
                \end{subfigure}
                \begin{subfigure}[b]{0.15\linewidth}
                    \includegraphics[width=\linewidth]{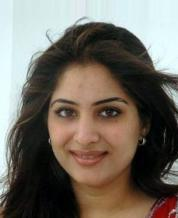}
                    
                \end{subfigure}
                \begin{subfigure}[b]{0.15\linewidth}
                    \includegraphics[width=\linewidth]{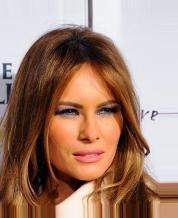}
                    
                \end{subfigure}
                \begin{subfigure}[b]{0.15\linewidth}
                    \includegraphics[width=\linewidth]{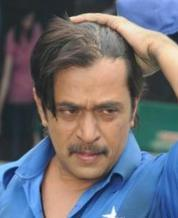}
                    
                \end{subfigure}
                \begin{subfigure}[b]{0.15\linewidth}
                    \includegraphics[width=\linewidth]{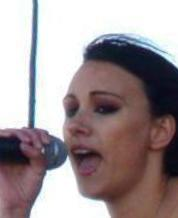}
                    
                \end{subfigure}
                \begin{subfigure}[b]{0.15\linewidth}
                    \includegraphics[width=\linewidth]{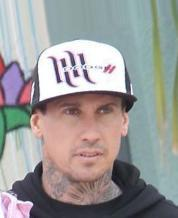}
                    
                \end{subfigure}
            \end{subfigure}
            \caption{Error samples of MSO=false in original dataset.}
        \end{subfigure}
        
    \end{subfigure}
   \caption{Error samples that are caused by the inconsistent definition.}
\label{fig:inconsistent-definition}
\end{figure}
