# Supplementary material for: Consistency and Accuracy of CelebA Attribute Values
Source: arXiv:2210.07356 source file (2023-04-16)
Supplement: Supplementary file 8 [file supplementary_material.tex]

\documentclass[10pt,twocolumn,letterpaper]{article}

\usepackage{cvpr}              %

\usepackage{graphicx}
\usepackage{amsmath}
\usepackage{amssymb}
\usepackage{booktabs}
\usepackage{xcolor}
\usepackage{algorithm}
\usepackage{algorithmic}
\usepackage{pifont}
\usepackage[utf8]{inputenc}
\usepackage{hhline}
\usepackage{color, colortbl}
\usepackage{multirow}
\usepackage{times}
\usepackage{epsfig}
\usepackage{lipsum} 
\usepackage{pythonhighlight}
\usepackage[accsupp]{axessibility}
\usepackage{makecell}
\usepackage{minted}
\usepackage{url}
\newcommand{\ra}[1]{\renewcommand{\arraystretch}{#1}}
\newcommand{\cmark}{\ding{51}}%
\newcommand{\xmark}{\ding{55}}%

\newcommand{\hw}[1]{\textcolor{blue}{\textit{HW: #1}}}
\renewcommand{\listingscaption}{Code}

\usepackage[pagebackref,breaklinks,colorlinks]{hyperref}
\setminted[python]{breaklines, framesep=2mm, fontsize=\footnotesize, numbersep=5pt}

\usepackage[capitalize]{cleveref}
\crefname{section}{Sec.}{Secs.}
\Crefname{section}{Section}{Sections}
\Crefname{table}{Table}{Tables}
\crefname{table}{Tab.}{Tabs.}

\def\cvprPaperID{1} %
\def\confName{CVPR}
\def\confYear{2023}


\begin{document}
\onecolumn


\begin{center}
{\bf Supplementary Material - Consistency and Accuracy of CelebA Attribute Values}\\
\end{center}
This supplementary material provides the examples of the errors in Section 3.3, which are caused by the short length of facial hair (Figure~\ref{fig:short-length-of-facial-hair}), less information (Figure~\ref{fig:information-lost}), and inconsistent definition (Figure~\ref{fig:inconsistent-definition}). Also, the examples of the third annotation option - information not visible - are shown in Figure~\ref{fig:imformation-not-visible}. In the CelebA dataset, there are some images that are not usable for face attribute classification, like corrupted image quality, face covered by the heavy face painting, multiple faces, etc. The examples are shown in Figure~\ref{fig:unusable-images}. As mentioned in Section 4.2, the edge images are difficult for people to mark them consistently, they are at the boundary of the definition, shown in Figure~\ref{fig:edge-images}. Finally, the Score-CAMs in Figure~\ref{fig:gradcams} are created to show where the networks look at when they predict the mouth slightly open (MSO). The CAMs show that both models look at the meaningful position when predicting MSO=True. However, when MOON-original predicts MSO=False, instead of looking at mouth, it looks at eye area. Our model looks at the correct position when it predicts MSO=False. Therefore, the cleaned annotations can guide the model to the correct direction.

\input{supplementary_marterial_figure_text_files/short_length_of_facial_hair}

\input{supplementary_marterial_figure_text_files/information_lost}

\input{supplementary_marterial_figure_text_files/inconsistent_definitions}

\input{supplementary_marterial_figure_text_files/information_not_visible}

\input{supplementary_marterial_figure_text_files/unusable_images}

\input{supplementary_marterial_figure_text_files/edge_images}

\input{supplementary_marterial_figure_text_files/gradcams}

\end{document}
